# Supplementary material for: Nano-scale magnetic skyrmions and target states in confined geometries
Source: arXiv:1901.06999 ancillary file (2019-05-17)
Supplement: Supplementary file 1 [file supplementary_material.pdf]

# Supplemental Material for: Nano-scale magnetic skyrmions and target states in confined geometries

David Cortés-Ortuño,[1,*] Niklas Romming,[2] Marijan Beg,[3] Kirsten von Bergmann,[2]
André Kubetzka,[2] Ondrej Hovorka,[1] Hans Fangohr,[1,3] and Roland Wiesendanger[2]

[1] *Faculty of Engineering and Physical Sciences, University of Southampton, Southampton SO17 1BJ, United Kingdom*
[2] *Institute of Applied Physics, University of Hamburg, Jungiusstrasse 11, D-20355 Hamburg, Germany*
[3] *European XFEL GmbH, Holzkoppel 4, 22869 Schenefeld, Germany*

## CONTENTS


S1. Sample preparation 3

S2. Magnetoresistance effects in scanning tunneling microscopy 3

S3. Edge tilt 4

S4. Boundary condition for $Pd_2$/Fe/Ir(111) 4

S5. Magnetic parameters 5

S6. Energies of iron palladium islands 6

S7. Simulation details 7

S8. Stability of target states 9

S9. Transition of a $3\pi$-skyrmion 10

S10. Hexagons: skyrmion energy 11

S11. Hexagons: Skyrmion as a function of island size 12

S12. Hexagons: skyrmion escape through the boundary 13

S13. Hexagons: transition of a target state 15

References 16

## S1. SAMPLE PREPARATION

The samples were prepared in-situ in a multi-chamber ultra-high vacuum system. The Ir(111) crystal was initially cleaned and depleted of carbon contamination by repeated annealing cycles in an oxygen atmosphere of $p(O_2)$ in the range of $1 \cdot 10^{-6}$ to $5 \cdot 10^{-8}$ mbar. During the cycles the crystal temperature was continuously increased via electron beam heating to $T_{max} \approx 1800\,\mathrm{K}$. To remove surface contaminations and deposited material, the crystal was sputtered with Ar-ions for approx. 10 min ($U_{acc} = 800\,\mathrm{V}$, $p(\mathrm{Ar}) \approx 9 \cdot 10^{-5}$ mbar, sputtering rate of around 3 monolayer (ML) per minute). Subsequently, the sample was annealed to about 1600 K for about 90 s to restore a smooth surface. Once the Ir(111) crystal is sufficiently clean and free of carbon contaminations in a depletion zone near the surface, the initial annealing in an oxygen atmosphere does not need to be repeated for every preparation procedure.

About 5 min after the annealing of the Ir substrate about $0.7 - 1.0$ ML of Fe were deposited by a standard electron-beam evaporator onto the warm surface at around 0.6 ML/min. This results mostly in self-organized step flow growth. The first layer of Fe grows pseudomorphically, continuing the face centered cubic (fcc) stacking of the substrate. When the Pd is deposited directly after the Fe deposition it forms extended islands consisting of a single Pd atomic layer with only small Pd DL islands on top; such a preparation was performed for the sample shown in Fig. 7. To obtain small monolayer high Pd islands directly on the Fe monolayer, as in Fig. 1, the Fe/Ir(111) sample was held at room temperature during Pd deposition. Subsequent gentle annealing leads to the roughly hexagonal island shape.

After the preparation the samples were transferred to a low-temperature ($T = 4.2\,\mathrm{K}$) ultra-high vacuum scanning tunneling microscope (STM) equipped with an external magnetic field perpendicular to the sample surface ($B \leq 9\,\mathrm{T}$). Topographic images were obtained in constant-current mode and maps of differential conductance ($\mathrm{d}I/\mathrm{d}U$) were measured simultaneously using lock-in technique. Spin-resolved measurements were performed using a Cr-bulk tip.

## S2. MAGNETORESISTANCE EFFECTS IN SCANNING TUNNELING MICROSCOPY

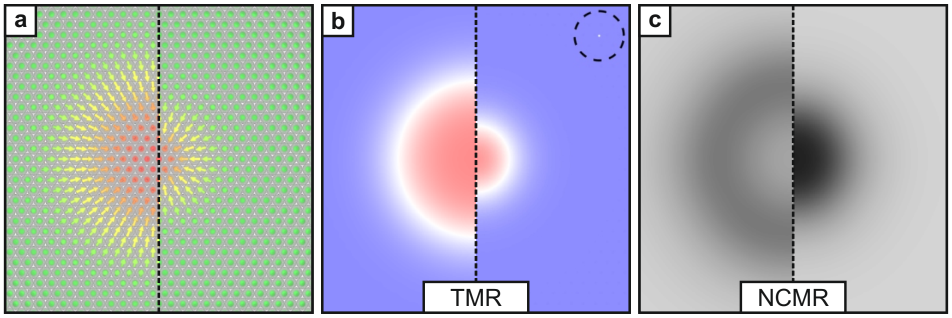


SUPP. FIG. S1. Magnetoresistance effects in STM. (a) Sketches of a larger and a smaller magnetic skyrmion, left and right, respectively; arrows indicate atoms and point in the direction of their magnetic moments, colors indicate their out-of-plane magnetization components. (b) expected TMR signal for a tip magnetized perpendicular to the sample surface, *i.e.* sensitive to the out-of-plane magnetization components of the sample. (c) expected NCMR signal also for non-magnetic tips, which scales with the degree of non-collinearity of the sample magnetization; whereas it is maximal (in this case darker) near the in-plane components of the sample magnetization for larger skyrmions, it has its maximum at the center for smaller skyrmions.

Spin-polarized STM exploits the tunnel magnetoresistance (TMR) effect between a magnetic tip and a magnetic sample, with the insulating vacuum tunnel barrier[1]. The TMR scales with the projection of tip and sample magnetization, *i.e.* the magnetic contribution to the signal is maximal for parallel or antiparallel tip and sample magnetization. A magnetic skyrmion, see sketch in Fig. S1(a), is imaged as a round object with a tip magnetized perpendicular to the surface, see (b), regardless of the size of the skyrmion (compare left and right side of the images for larger/smaller skyrmion in lower/higher external applied field). Due to spin mixing of the electronic states in non-collinear spin textures, their vacuum density of states is different compared to that of collinear magnetic states. This difference can be detected also with non-magnetic tips and manifests in the non-collinear magnetoresistance (NCMR)[2] effect, see Fig. S1(c). The NCMR signal scales roughly with the angle between nearest neighbor magnetic moments and the appearance of skyrmions changes from ring-like for larger skyrmions to dot-like for small skyrmions. A spin spiral appears as stripes both in TMR as well as in NCMR, but in NCMR the measured wavelength is half of that of the magnetic period.

## S3. EDGE TILT

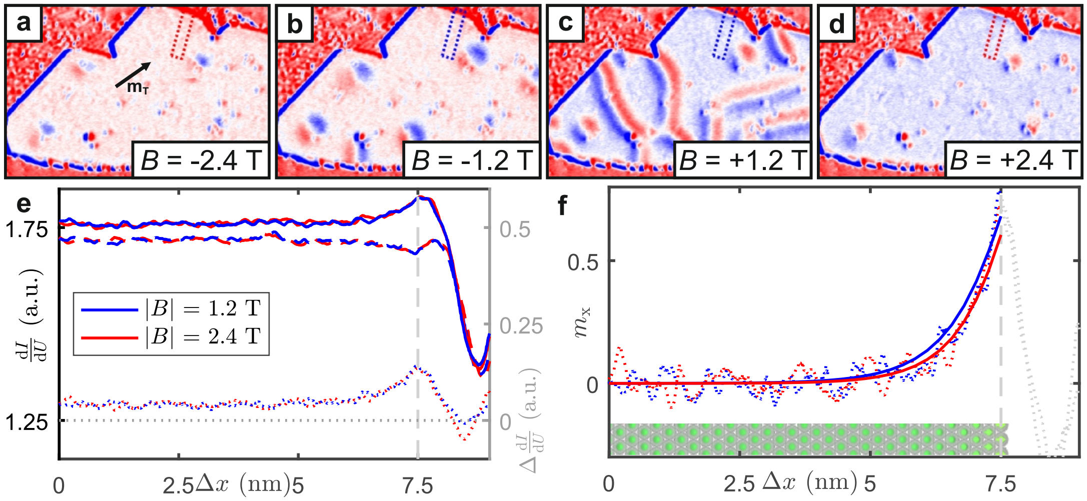


SUPP. FIG. S2. Edge tilt in hcp Pd/Fe/Ir(111). (a)-(d) Spin-resolved $\mathrm{d}I/\mathrm{d}U$ maps of the same Pd/Fe/Ir(111) island at the indicated applied magnetic fields measured with a dominantly in-plane magnetized tip that does not react to applied magnetic fields. (e) Line profiles along the dotted rectangles in (a)-(d) (solid lines: positive magnetic field, dashed lines: negative magnetic field). Dotted lines show the respective difference between the line profiles at the two different $|B|$. (f) Calculated magnetization component along the profile direction $m_x$ as dotted lines. For the calculation of $m_x$, the tip magnetization direction $m_T$ was determined by 2-dimensional fits to the skyrmions[3] resulting in a polar angle $\theta = 78^\circ$ and an azimuthal angle $\phi = 40^\circ$ relative to the direction of the line profiles (see also arrow in (a) for $m_T$); the solid lines represent the $m_x$-component of simulated data; inset at the bottom shows top view representation of spins at $B = 1.2\,\mathrm{T}$, corresponding to the blue solid line.

## S4. BOUNDARY CONDITION FOR $PD_2$/FE/IR(111)

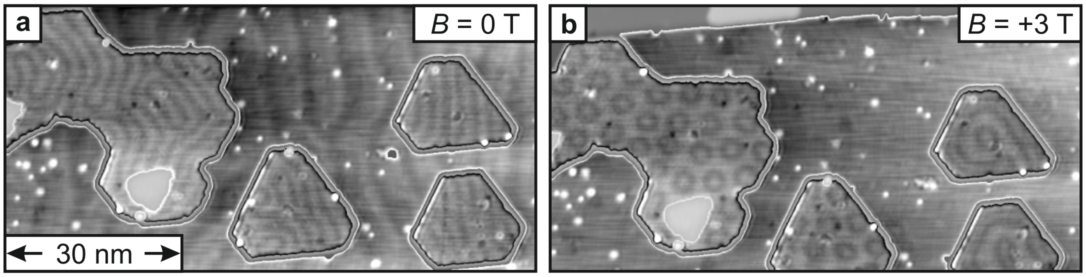


SUPP. FIG. S3. (a),(b) (SP-)STM topography images of $Pd_2$/Fe islands surrounded by a Pd/Fe film on Ir(111), where the NCMR signal is dominant for the $Pd_2$/Fe islands and the TMR dominates the signal for the Pd/Fe film; the gray-scale is adjusted individually for the islands and the film to $\pm 10\,\mathrm{pm}$; Gauß-filtered in the vertical direction with $\sigma = 1.2\,\text{Å}$; Cr-bulk tip, $T = 4.2\,\mathrm{K}$, $I = 1\,\mathrm{nA}$, $U = +50\,\mathrm{mV}$. (a) The Pd double layer islands on Fe/Ir(111) exhibit a spin spiral ground state at zero applied magnetic field with a period of about 4.5 nm; they are typically surrounded by Pd monolayer on Fe/Ir(111) areas, with a spin spiral of about 7 nm. (b) Both magnetic states undergo several phase transitions, but the critical fields differ for the two systems: at an applied magnetic field of +3 T, the $Pd_2$/Fe hosts many skyrmions, whereas the surrounding Pd/Fe is mostly ferromagnetic, thus imposing a ferromagnetic boundary condition on the $Pd_2$/Fe islands. The magnetic state of the two $Pd_2$/Fe islands to the right can be interpreted as follows: the rim of the island is magnetized up (parallel to the magnetic field aligned Pd/Fe film), the outer dark line marks a rotation of the magnetization to the other out-of-plane magnetization direction, *i.e.* down, and the inner ring again shows a rotation of the magnetic texture and thus the magnetization in the center is again up; thus the spin texture of the $Pd_2$/Fe resembles target skyrmions.

## S5. MAGNETIC PARAMETERS

From Ref. 3 the micromagnetic parameters for a Pd/Fe/Ir(111) system are

| | | |
|---|---|---|
| Exchange constant | $A$ | 2 pJ m$^{-1}$ |
| DMI constant | $D_\mathrm{c}$ | 3.9 mJ m$^{-2}$ |
| Anisotropy constant | $K$ | 2.5 MJ m$^{-3}$ |
| Saturation magnetization | $M_\mathrm{s}$ | 1.1 MA m$^{-1}$ |

We convert these parameters to the discrete spin model. By taking into account a monolayer of spins with a triangular lattice geometry, lattice constant $a$ and thickness $a_z$, we use the following formulae

$$A = \frac{\sqrt{3}J}{2a_z} \qquad D_\mathrm{c} = \frac{\sqrt{3}D}{a a_z} \qquad M_\mathrm{s} = \frac{\mu}{\frac{\sqrt{3}}{2}a^2 a_z} \qquad K = \frac{\mathcal{K}}{\frac{\sqrt{3}}{2}a^2 a_z} \tag{1}$$

Using a thickness and lattice constant from Refs.3 and 4, the atomistic parameters are calculated as

| | | |
|---|---|---|
| Lattice constant | $a$ | 2.715 Å |
| Thickness | $a_z$ | 4.08 Å |
| Exchange constant | $J$ | 5.88 meV |
| DMI constant | $D$ | 1.56 meV |
| Anisotropy constant | $\mathcal{K}$ | 0.41 meV |
| Magnetic moment | $\mu$ | 3 $\mu_\mathrm{B}$ |

## S6. ENERGIES OF IRON PALLADIUM ISLANDS

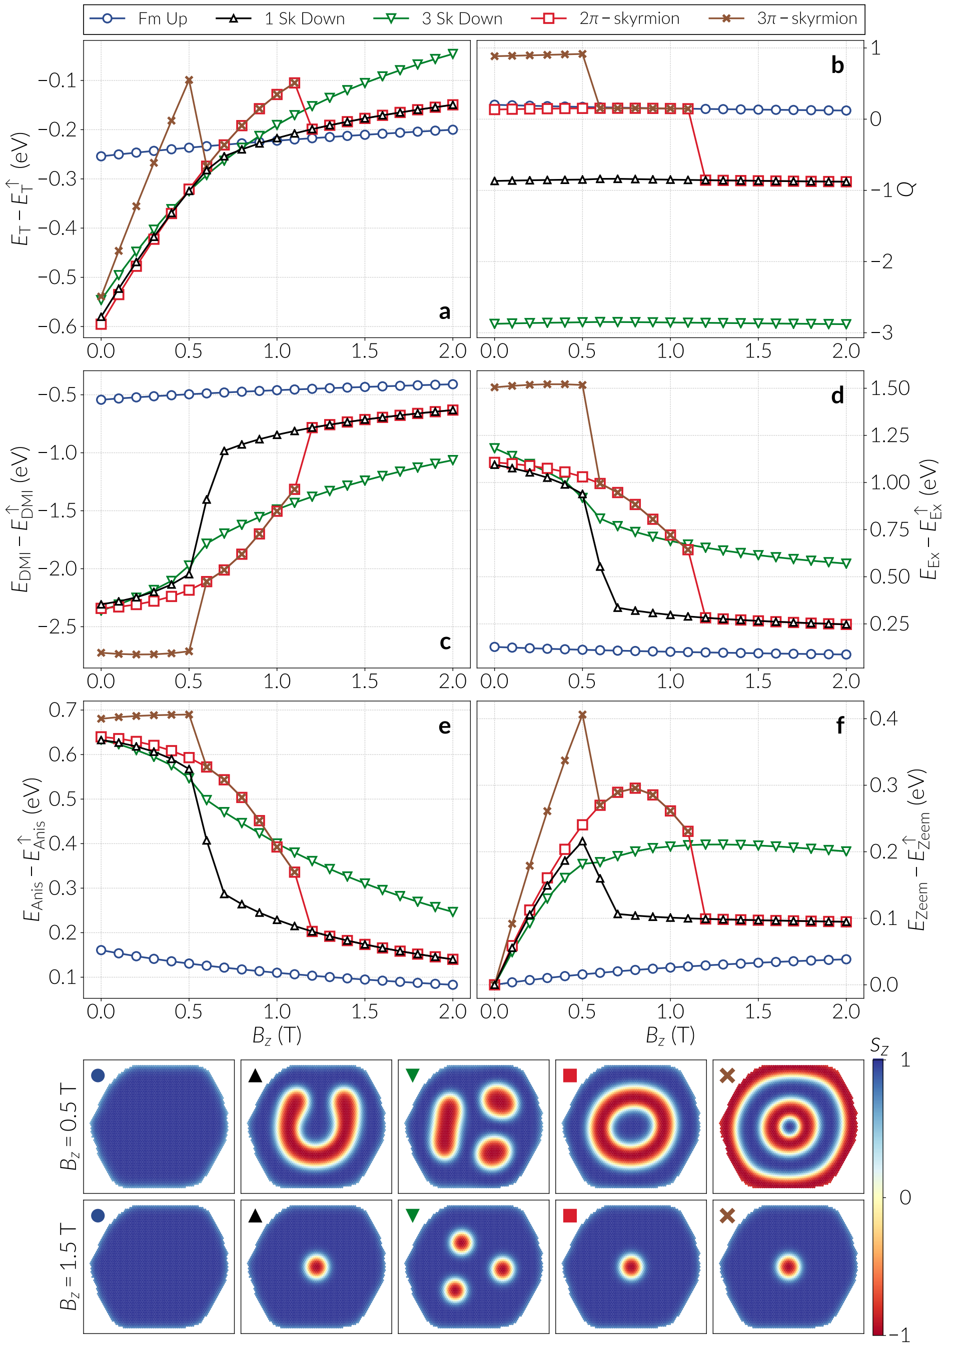


SUPP. FIG. S4. Magnetic energies and topological charge of five different magnetic configurations: ferromagnetic ordering, (Fm up), a single skyrmion (1 Sk Down), three skyrmions (3 Sk Down), a target state, and a 3$\pi$-skyrmion. Snapshots of these states under a field of $B_z = 0.5\,\mathrm{T}$ and $B_z = 1.5\,\mathrm{T}$ are shown at the two bottom rows of the figure, where the color scale refers to the out-of-plane spin component $s_z$. Every plot is shown as a function of the applied magnetic field, which points in the $z$ direction of the sample. Energies are computed with respect to a fully saturated state (denoted by $\uparrow$) at corresponding magnetic field strengths. (a) Total energy. (b) Topological charge. (c) Dzyaloshinskii-Moriya interaction energy. (d) Exchange interaction energy. (e) Anisotropy energy. (f) Zeeman interaction energy.

## S7. SIMULATION DETAILS

For the relaxation of the systems we use the Landau-Lifshitz-Gilbert (LLG) equation. Numerically, it is necessary to fix the length of the magnetization, which changes due to the effect of error propagation during integration. Therefore we add a corrector term to the LLG equation to keep the spin length $|\mathbf{s}|$ as a unit. According to this, our discrete spin code is implemented with the following LLG equation

$$\frac{\partial \mathbf{s}}{\partial t} = -\gamma \, \mathbf{s} \times \mathbf{H}_{\mathrm{eff}} + \frac{\alpha_{\mathrm{G}}\gamma}{\mu} \, \mathbf{s} \times \mathbf{s} \times \mathbf{H}_{\mathrm{eff}} + c\sqrt{\left(\frac{\partial \mathbf{s}}{\partial \tau}\right)^{2}} \left(1 - \mathbf{s}^{2}\right) \mathbf{s} \,, \tag{2}$$

where $\mathbf{H}_{\mathrm{eff}}$ is the effective field, $\gamma$ is the gyromagnetic ration, which sets the time scale of the integration, and $c$ is a weight for the corrector term. In most cases we are not interested in the dynamics of a system, thus we set $\gamma = 1$ and accelerate the minimization by removing the precessional term (first term to the right hand side) of Equation 2 and setting an appropriate damping value.

To stop the minimization process it is necessary to set a stopping criteria for the integration of Equation 2, thus at every time step $t$ we estimate the maximum value of the time derivative among all spins $\mathbf{s}$ using the time of the previous time step $t_{\mathrm{prev}}$, *i.e.* we calculate

$$\Delta s = \max \left| \frac{\mathbf{s}(t) - \mathbf{s}(t_{\mathrm{prev}})}{t - t_{\mathrm{prev}}} \right| . \tag{3}$$

If $\Delta s$ is less than a specific threshold value $\Delta s_{\mathrm{th}}$, we stop the minimization process. In the main study we specify a strict tolerance by setting threshold values between $\Delta s_{\mathrm{th}} = 10^{-5}$ and $\Delta s_{\mathrm{th}} = 10^{-6}$, and using a damping of magnitude $\alpha_{\mathrm{G}} = 0.01$. Larger threshold values, *i.e.* a weaker tolerance, with smaller damping values can stop the relaxation at unstable or metastable states. For example, in Fig. S5 we show the relaxation of a skyrmion and a $3\pi$-skyrmion in a hexagonal island, which are shown in Fig. 3 of the main study, using $\Delta s_{\mathrm{th}} = 10^{-4}$ and $\alpha_{\mathrm{G}} = 0.001$. We notice that using a weak tolerance the simulations relax into a bubble-like configuration, whose energy follows the tendency of the curve for fields below 0.7 T. This is in contrast to the jump in the energy curve for the tolerances used in the paper. In the case of the $3\pi$-skyrmion configuration, this state can be stabilized up to a slightly larger field value of 0.7 T, compared to the paper result. Afterwards, it relaxes into the $2\pi$-skyrmionup to a field of 1.3 T, which is again a slightly larger critical field than the one shown in the paper. The problem of using weak tolerances is that there is no guarantee that the configuration being stabilized is sitting exactly at a local minimum, and the energy found by the algorithm is usually larger than the expected value from a completely relaxed configuration (see, for example the energy values of the $3\pi$-skyrmion state when using a weak tolerance in Fig. S5). At the range of field magnitudes for the skyrmion states, obtained from using a weak tolerance, the barrier separating the local minimum (at which the LLG equation is relaxing to) from an energetically close state is significantly small (see, for instance, Fig. S6). In addition, it becomes difficult to find specific combinations for the damping and tolerance $\Delta s_{\mathrm{th}}$ to avoid that the algorithm overcomes the barrier separating the metastable state being relaxed and finds a lower energy configuration. Accordingly, we decided to use a small value for $\Delta s_{\mathrm{th}}$ in order to be sure that the configuration being found is sitting at a true local energy minimum.

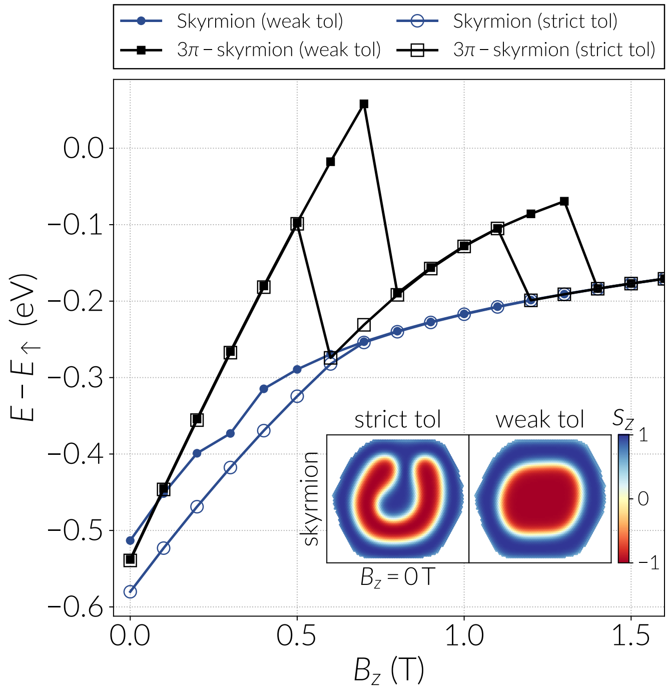


SUPP. FIG. S5. Energy of a skyrmion and a $3\pi$-skyrmion configuration in a hexagonal island of Pd/Fe/Ir(111), as a function of the applied field. The plot shows the results obtained from relaxations using a weak tolerance (weak tol) for stopping the minimization ($\Delta s_{\mathrm{th}} = 10^{-4}$, $\alpha_{\mathrm{G}} = 0.001$), and the tolerance from the results shown in the paper. Snapshots of the skyrmion configuration at zero field, for both tolerances, are depicted in the inset images.

## S8. STABILITY OF TARGET STATES

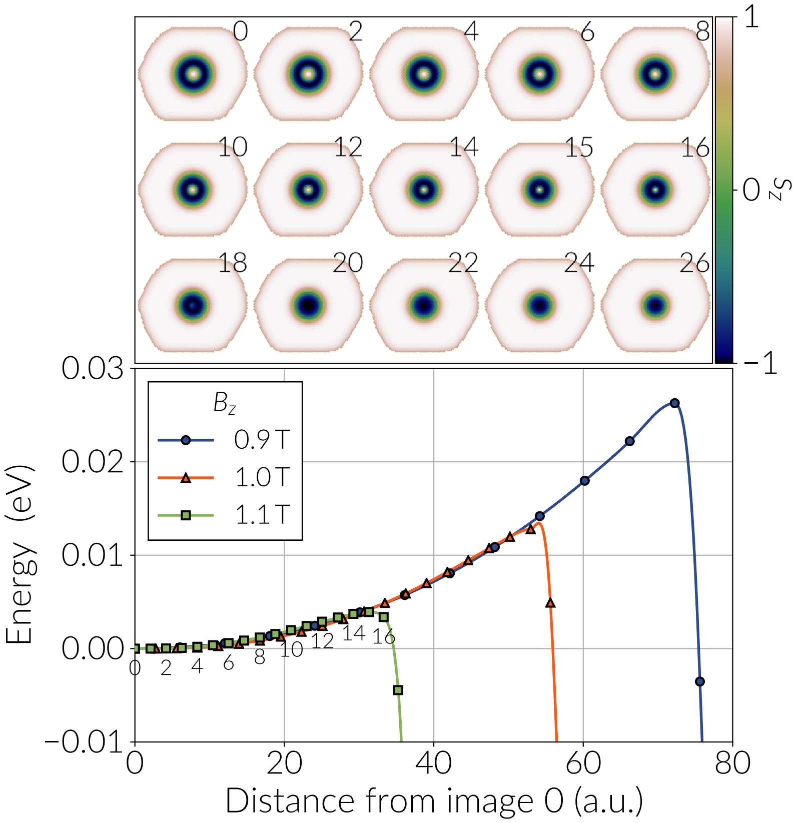


SUPP. FIG. S6. Target state collapse into a skyrmion. Minimum energy path between a target state and a skyrmion in a Pd/Fe/Ir(111) island for three external field magnitudes. The curves in the lower plot refer to the energy bands[5], which are only shown with the first few images and where the target state is the data point at the leftmost side of the bands. The energy scale is shifted with respect to the target state energy. The figure at the top shows snapshots of the images for the $B_z = 1.1\,\mathrm{T}$ case, where the numbers at every snapshot correspond to the numbers in the data points of the curve. The colormap refers to the out-of-plane component of the spins.

In Fig. 3(a) of the main study we observe that target states in Pd/Fe/Ir(111) islands cannot be stabilized above a field of $B_z = 1.1\,\mathrm{T}$ since the system relaxes to an isolated skyrmion. One possible reason for this instability is that the energy barrier separating these two configurations is reduced as the magnetic field increases, thus a target state would decay above a critical field. Under this hypothesis we performed a stability calculation between a target state and a skyrmion by means of the GNEBM.[6,7] By specifying the target state and the skyrmion as the initial and final state in an energy band[5], respectively, and initializing the energy band with a linear interpolation, the resulting transition after relaxation is depicted in Fig. S6 for three different magnetic fields, $B_z = 1.1$, 1.0 and $0.9\,\mathrm{T}$. We confirm from this figure that the energy barrier decreases as we increase the magnetic field. At the top of Fig. S6 we show snapshots of the images of the band with $B_z = 1.1\,\mathrm{T}$, whose curve is numbered. The sequence shows a collapse of the target state into a skyrmion, where the saddle point is given when the inner core of the target state reverts to give rise to the skyrmion core, which points in the $-z$ direction. Since we could not relax a target state at $B_z = 1.2\,\mathrm{T}$ (it might be possible using a weak tolerance for the relaxation of the target state), the critical field must lie between $B_z = 1.1\,\mathrm{T}$ and 1.2 T. For a field of $B_z = 0.8\,\mathrm{T}$, which we do not show here, we saw that the energy barrier is significantly larger, around 0.06 eV, although the transition is mediated by a singularity[7] rather than by a collapse. We observed a similar phenomenon for the transition between a $3\pi$-skyrmion and a $2\pi$-skyrmion, which is shown in Sec. S9.

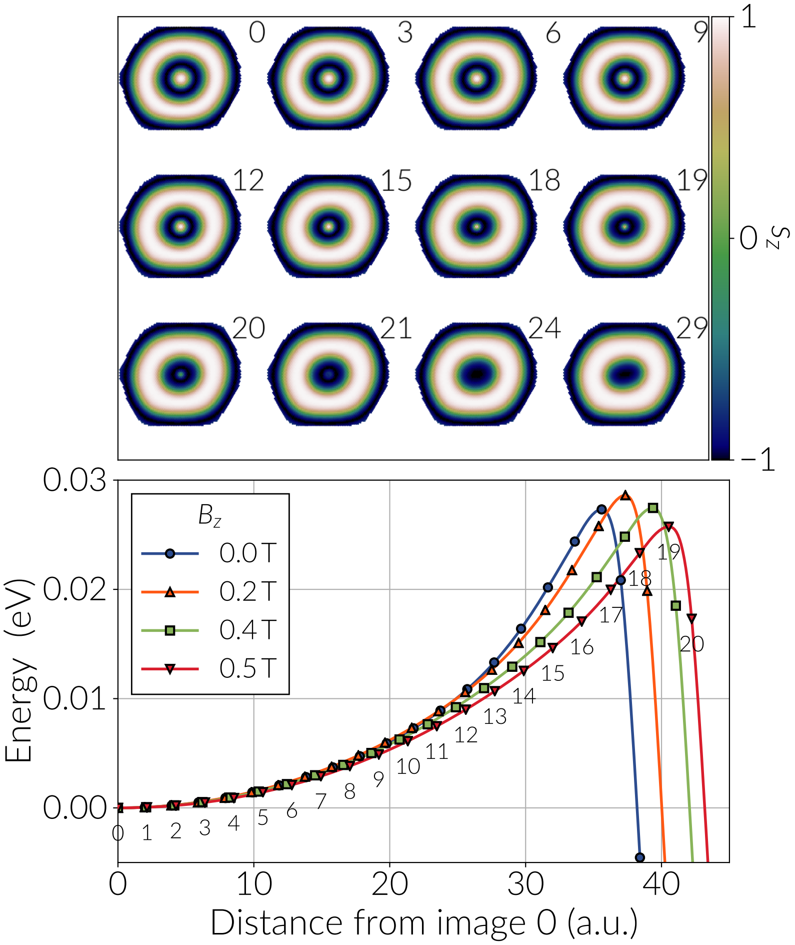


SUPP. FIG. S7. Energy bands for the transition of a $3\pi$-skyrmion configuration into a target state, as a function of the applied field. The main plot shows the first few images of the GNEBM energy bands[5], where the leftmost image in every band refers to the $3\pi$-skyrmion state. Energy magnitudes are shifted with respect to the energy of this configuration. The target state defined in these transitions has its core pointing in the opposite direction of the applied field. Snapshots above the main plot depict the transition at an applied field of 0.5 T, where numbers at the top right of every image correspond to the numbers in the curve.

## S9. TRANSITION OF A $3\pi$-SKYRMION

In Fig. S7 we illustrate the transition of a $3\pi$-skyrmion configuration into a $2\pi$-skyrmion, or target state, for different magnetic field values. This minimum energy path is given by the collapse of the inner core of the $3\pi$-skyrmion, which is similar to the transition of a $2\pi$-skyrmion into a skyrmion (see Fig. S6 in the main text). We notice from Fig. S7 that around a magnitude of 0.2 T the energy barriers, given by the largest energy points in every band, start to decrease. In the main study we found that a $3\pi$-skyrmion could not be stabilized for field values above 0.5 T. Although it might be possible to extend this critical value by using weaker tolerances in the minimization, as explained in Sec. S7, configurations found with this criteria are highly unstable. Target states shown in the transitions of Fig. S7 have the core pointing in the opposite direction of the applied field, thus they are stable in a different range than target states with the core in the field direction, which are shown in Fig. 3 of the main text. A thorough analysis of the transitions related to skyrmion states is beyond the scope of the paper.

## S10. HEXAGONS: SKYRMION ENERGY

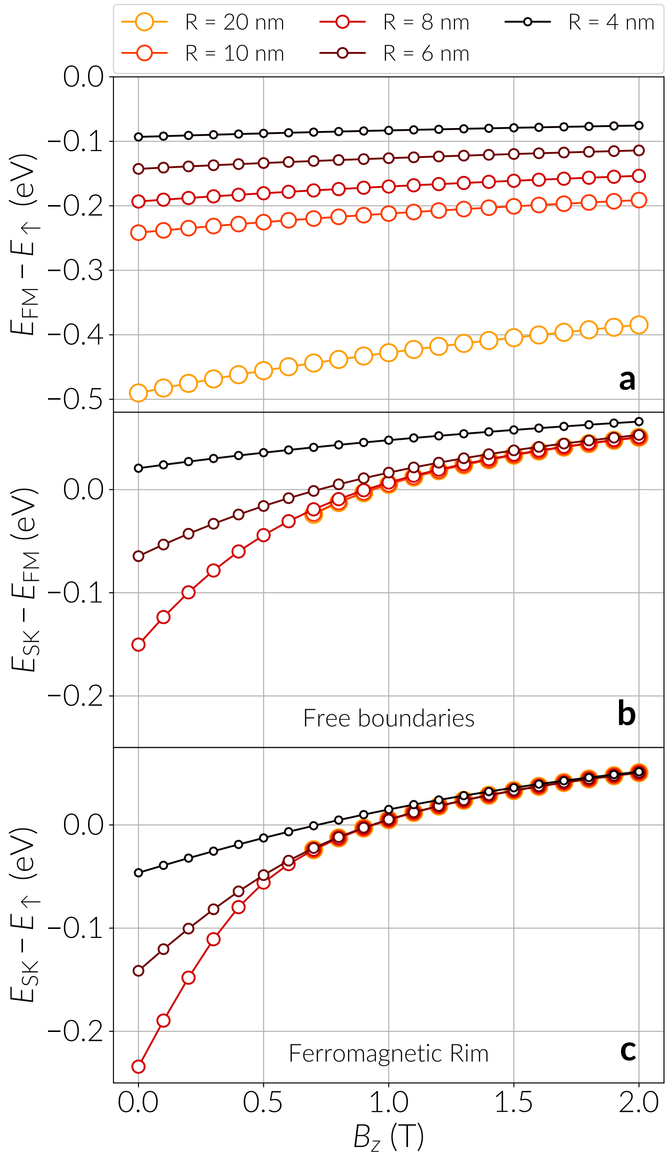


SUPP. FIG. S8. Energy of the ferromagnetic boundary and skyrmions in Pd/Fe/Ir(111) hexagons for different sizes and boundary conditions. (a) The curve refers to the energy of the ferromagnetic state $E_{\mathrm{FM}}$ with respect to the energy of the fully aligned configuration (in the $+z$ direction) $E_{\uparrow}$, as a function of the applied field. (b) Energy $E$ of the skyrmion with respect to the energy of the ferromagnetic state, as a function of the applied field, in hexagons with free boundaries. (c) Energy of the skyrmion and the target state with respect to the fully uniform configuration in hexagons with a ferromagnetic rim (the ferromagnetic state in this case corresponds to the fully aligned configuration).

## S11. HEXAGONS: SKYRMION AS A FUNCTION OF ISLAND SIZE

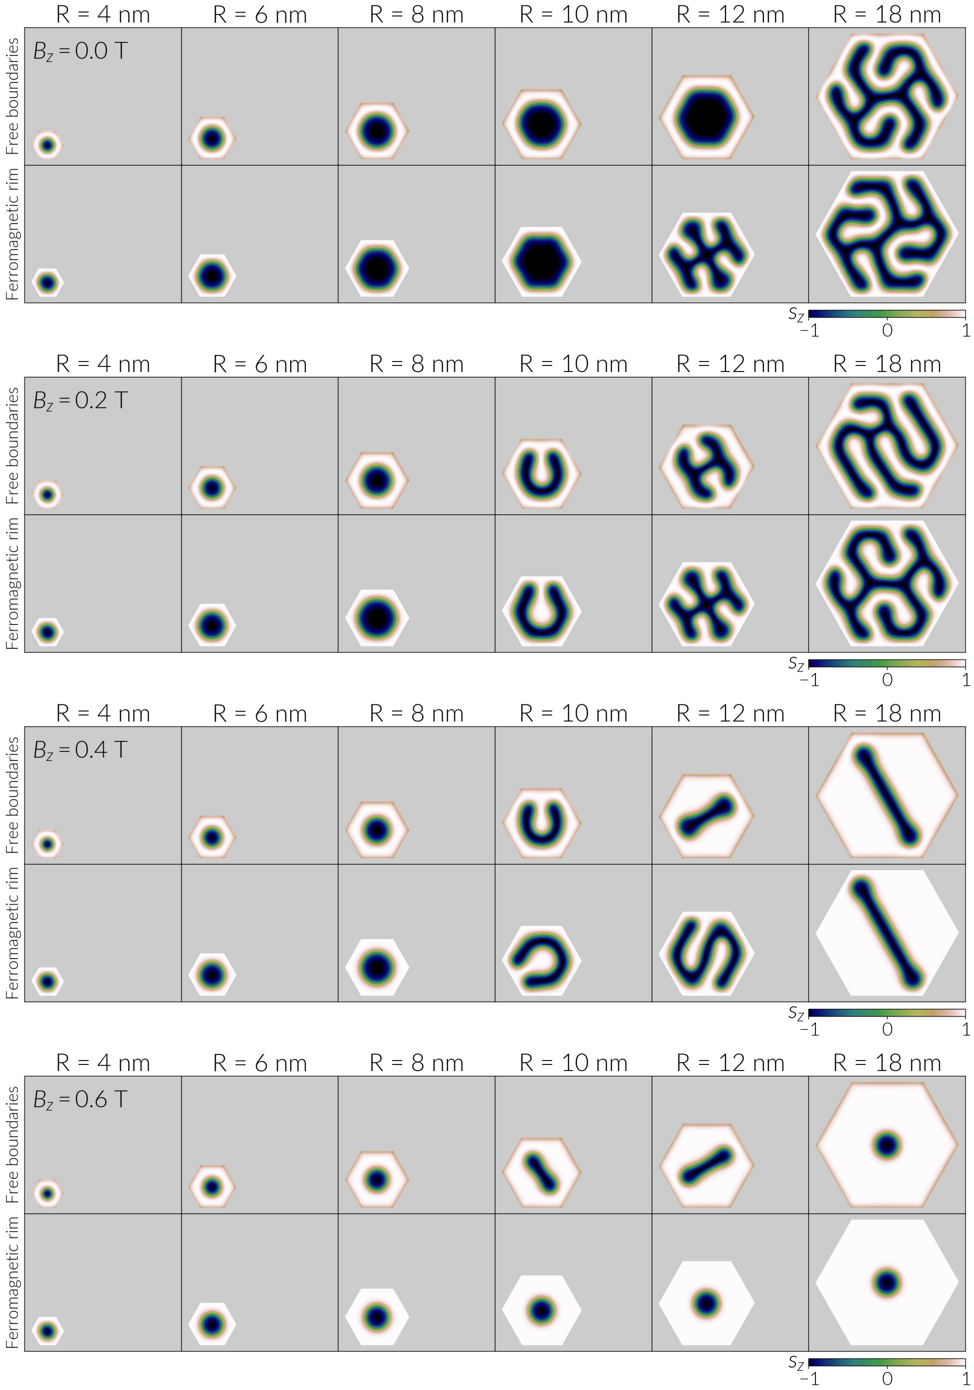


SUPP. FIG. S9. Relaxation of skyrmion configurations in Pd/Fe/Ir(111) hexagonal islands of different size, applied field and boundary condition. The size of the island is measured by the hexagon circumradius $R$. The field magnitude is shown at the top left of every set of snapshots. The first row of every set refers to islands with free boundaries and the second row to islands with a ferromagnetic rim.

## S12. HEXAGONS: SKYRMION ESCAPE THROUGH THE BOUNDARY

In the main study we analyze energy barriers between a skyrmion and the uniform state in hexagons of different size. These energy barriers are obtained by calculating minimum energy transitions between these two equilibrium configurations, using the Geodesic Nudged Elastic Band Method[6] (GNEBM). In Fig. S10 we show energy bands[5] after relaxation with the GNEBM, for the escape transition of skyrmions in hexagons of four different circumradii $R$ and a few applied field values. The energy scale in these bands is shifted with respect to the skyrmion energy at corresponding hexagon size and applied field. The continuous curves in these plots are given by a cubic polynomial

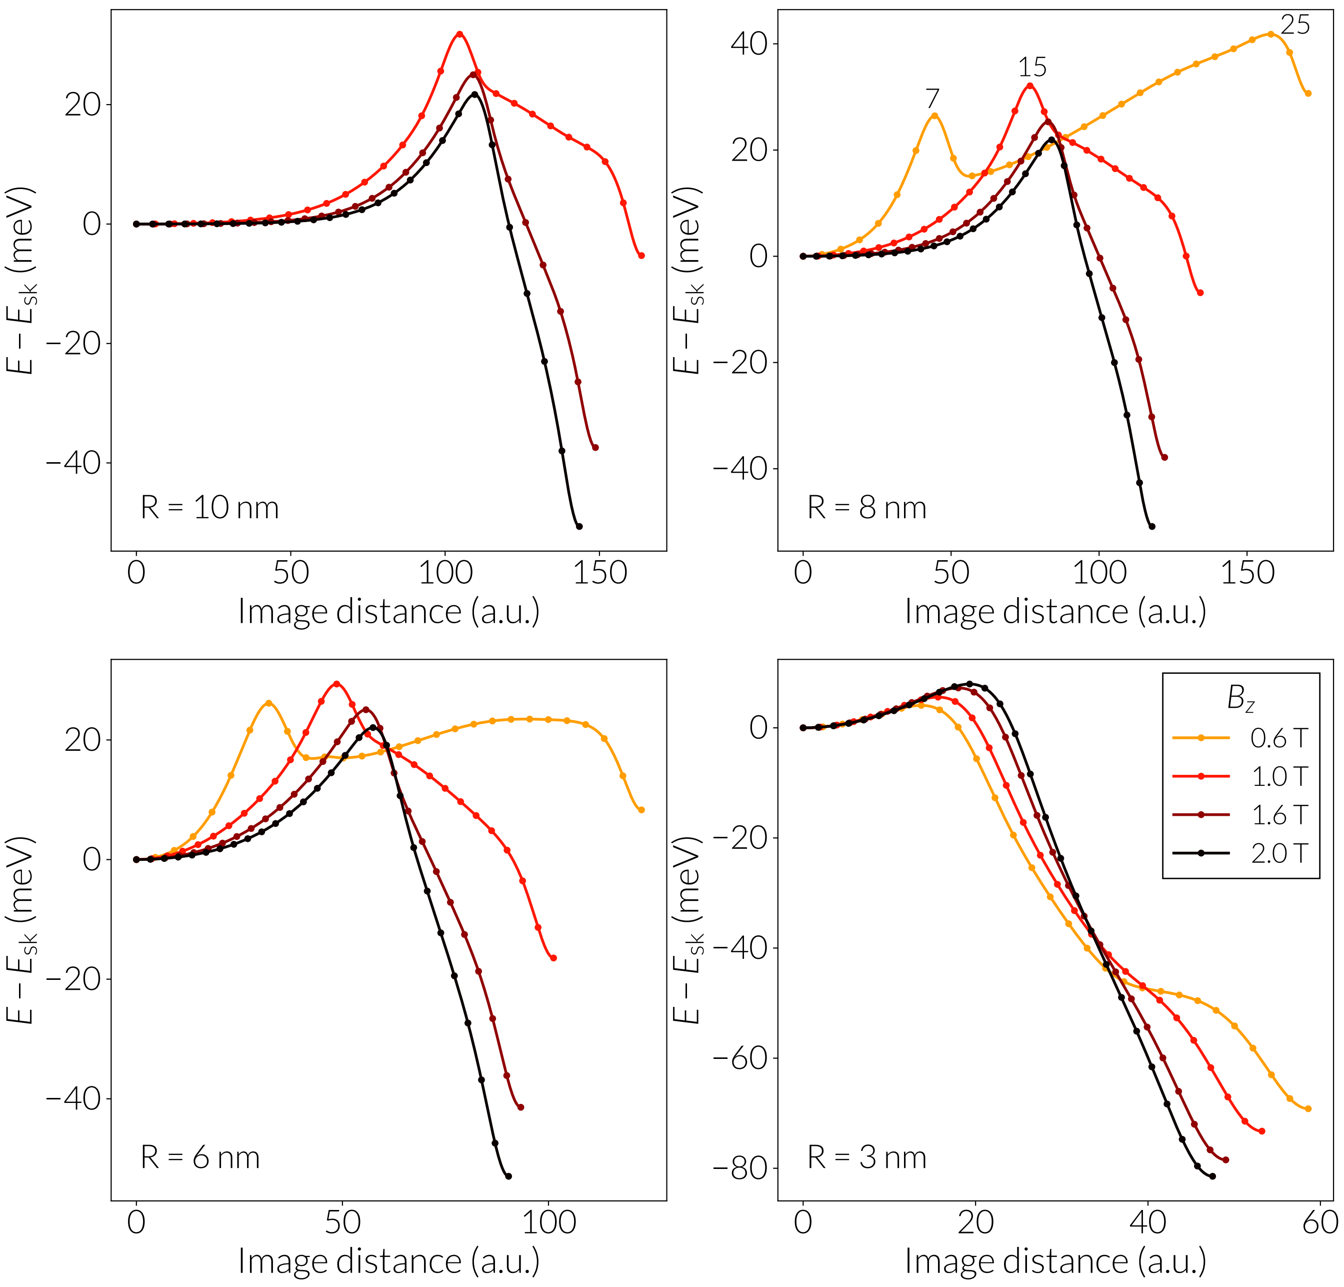


SUPP. FIG. S10. Energy bands for the escape transition of a skyrmion through the boundary of hexagons of different size, as a function of the magnetic field strength. The hexagon size is specified by its circumradius $R$, which is shown at the bottom left of every plot. Energy scales are shifted with respect to the skyrmion energy. Energy bands were obtained with the GNEBM. The leftmost data point refers to the skyrmion state. Image numbers are shown at the saddle points of the $R = 8\,\text{nm}$ case for fields of 0.6 T and 1.0 T.

fit to the band images[6].

From the bands of Fig. S10 it can be noticed that at weak magnetic field magnitudes, which is 0.6 T in the energy band plots, the skyrmion energy is smaller than the uniform state energy. Moreover, from the plot of the $R = 8\,\mathrm{nm}$ case at this weak field the GNEBM finds two saddle points, which are numbered in the corresponding energy band. In this transition the skyrmion elongates until reaching the hexagon boundary before starting to escape through the boundary of the island. Snapshots of the images for the energy band[5] of this energy path are depicted in Fig. S11, where the saddle points are given by the 7th and 25th images. In the former, an elongated skyrmion reaches the top hexagon boundary, in the latter the skyrmion is about to escape from the top boundary. The energy barrier in this case is given by the saddle point with largest energy. By increasing the field the skyrmion decreases in size and the transition is given by the skyrmion displacement without distortion before reaching the boundary. In this case the energy band has a single saddle point. We mark this saddle point for the $R = 8\,\mathrm{nm}$ and 1.0 T case in Fig. S10, which is given by the 15th image, and snapshots of this energy path are shown in Fig. S12.

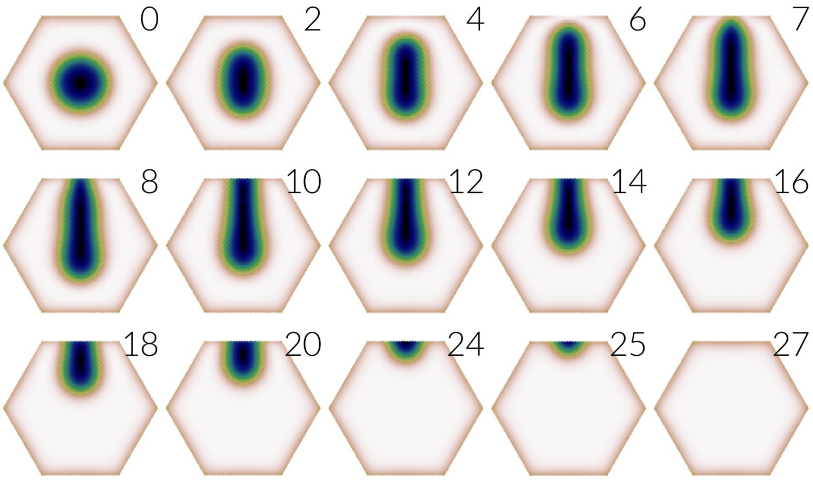


SUPP. FIG. S11. Snapshots for the skyrmion escape transition for $R = 8\,\mathrm{nm}$ and $B_z = 0.6\,\mathrm{T}$.

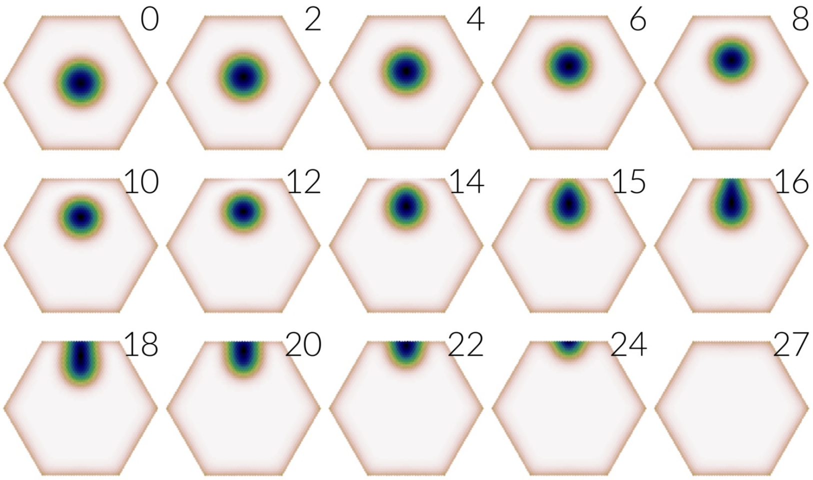


SUPP. FIG. S12. Snapshots for the skyrmion escape transition for $R = 8\,\mathrm{nm}$ and $B_z = 1.0\,\mathrm{T}$.

## S13. HEXAGONS: TRANSITION OF A TARGET STATE

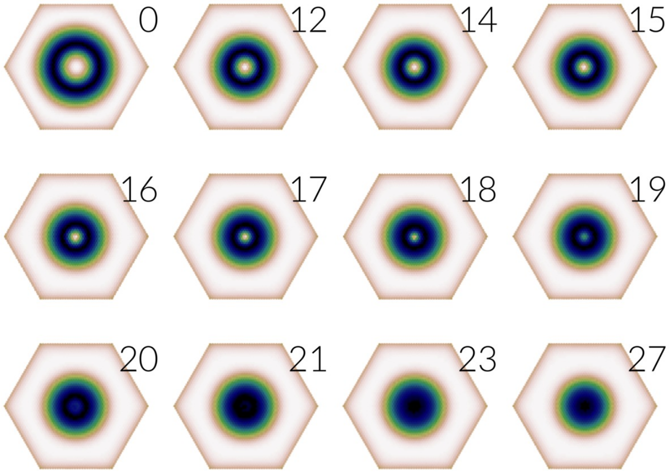


SUPP. FIG. S13. Snapshots for the transition of a target state into a skyrmion in a hexagonal island of size $R = 8\,\mathrm{nm}$ under an applied field of $B_z = 0.6\,\mathrm{T}$.

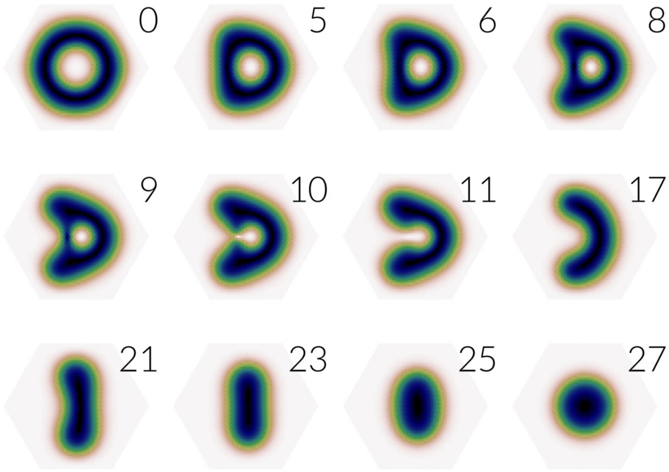


SUPP. FIG. S14. Snapshots for the transition of a target state into a skyrmion in a hexagonal island of size $R = 8\,\mathrm{nm}$ with ferromagnetic boundaries, under an applied field of $B_z = 0.6\,\mathrm{T}$.

* d.cortes@soton.ac.uk

[1] R. Wiesendanger, Rev. Mod. Phys. **81**, 1495 (2009).
[2] C. Hanneken, F. Otte, A. Kubetzka, B. Dupé, N. Romming, K. von Bergmann, R. Wiesendanger, and S. Heinze, Nature Nanotechnology **10**, 1039 (2015).
[3] N. Romming, A. Kubetzka, C. Hanneken, K. von Bergmann, and R. Wiesendanger, Phys. Rev. Lett. **114**, 177203 (2015).
[4] B. Dupé, M. Hoffmann, C. Paillard, and S. Heinze, Nature Communications **5**, 4030 (2014).
[5] An energy band is a sequence of copies of the system, each one in a different magnetic configuration and known as an image, along the transition path. The configurations at the extrema of the band are the equilibrium states between which the transition is being computed.
[6] P. F. Bessarab, V. M. Uzdin, and H. Jónsson, Computer Physics Communications **196**, 1 (2015).
[7] D. Cortés-Ortuño, W. Wang, M. Beg, R. A. Pepper, M.-A. Bisotti, R. Carey, M. Vousden, T. Kluyver, O. Hovorka, and H. Fangohr, Scientific Reports **7**, 4060 (2017).
